# Supplementary material for: Flux periodic oscillations and phase-coherent transport in GeTe nanowire-based devices
Source: arXiv:2009.06995 source file (2020-09-15)
Supplement: Supplementary file 1 [file GeTe-nanoribbons-SI-arXiv.pdf]

# Flux periodic oscillations and phase-coherent transport in GeTe nanowire-based devices

(Supplementary Information)

Jin-Zhong Zhang,[1, 2, 3] Pok-Lam Tse,[4] Abdur Rehman Jalil,[1, 2] Jonas Kölzer,[1,2] Daniel Rosenbach,[1,2] Martina Luysberg,[5] Gregory Panaitov,[6] Hans Lüth,[1,2] Detlev Grützmacher,[1,2] Zhigao Hu,[3,] Jia Grace Lu,[4] and Thomas Schäpers[1, 2,*]

[1]Peter Grünberg Institut (PGI-9), Forschungszentrum Jülich, 52425 Jülich, Germany

[2]JARA-Fundamentals of Future Information Technology, Jülich-Aachen Research Alliance, Forschungszentrum Jülich and RWTH Aachen University, Germany

[3]Key Laboratory of Polar Materials and Devices (MOE) and Technical Center for Multifunctional Magneto-Optical Spectroscopy (Shanghai), Department of Materials, School of Physics and Electronic Science, East China Normal University, Shanghai 200241, China.

[4]Department of Physics and Astronomy and Department of Electrophysics, University of Southern California, CA 90089, Los Angeles, USA

[5]Ernst Ruska Center, Forschungszentrum Jülich, 52425 Jülich, Germany

[6]Institute of Complex Systems (ICS-8) Forschungszentrum Jülich, 52425 Jülich, Germany

* email: th.schaepers@fz-juelich.de

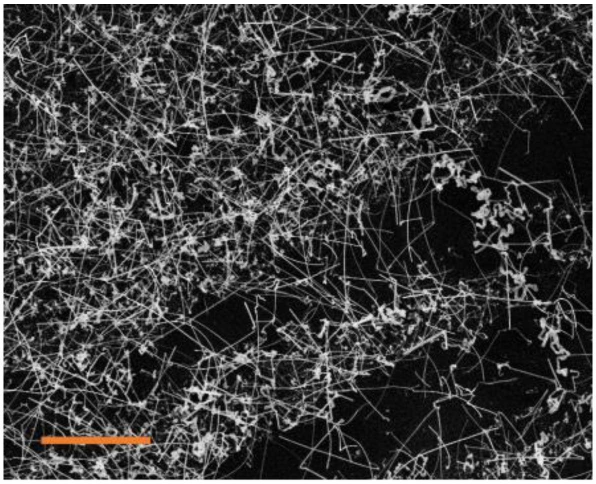

Figure S1. Scanning electron micrograph (SEM) image of the as-grown GeTe nanowires on $Si/SiO_2$ substrates. The scale bar corresponds to 5µm.

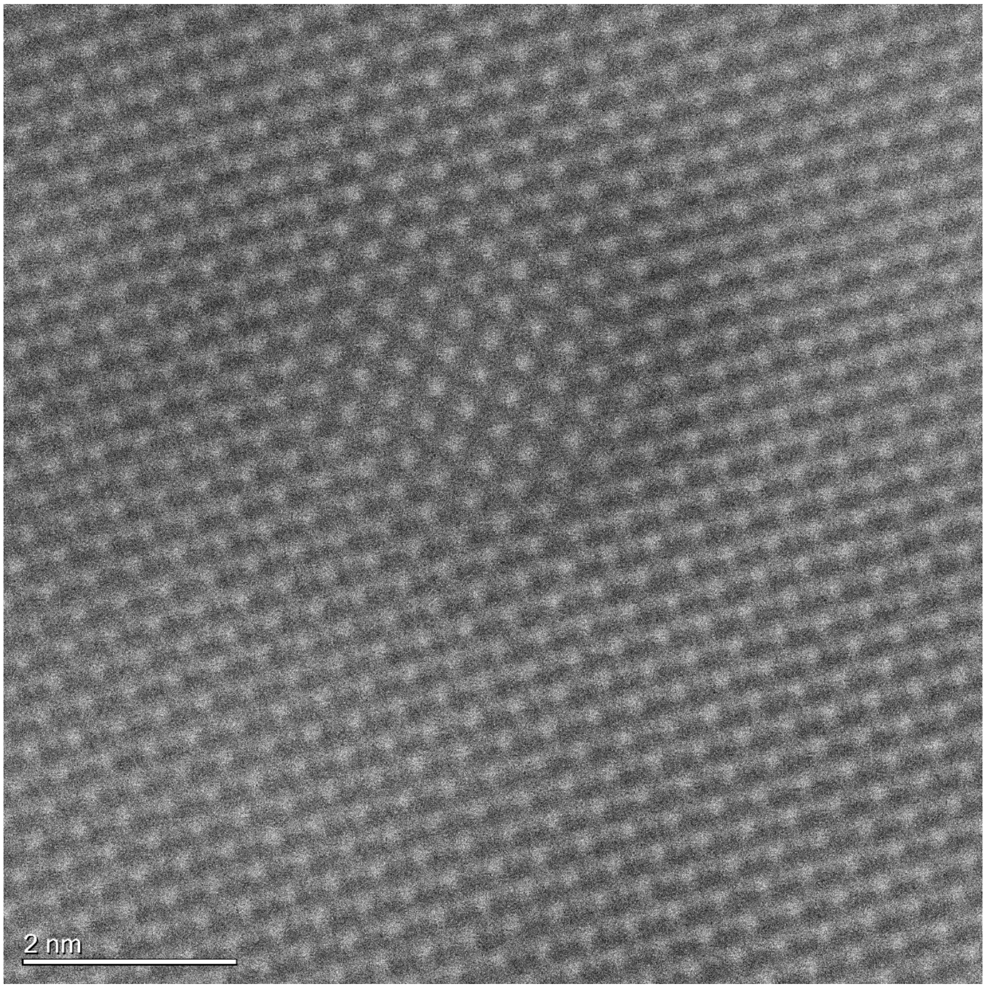


Figure S2. HAADF image of GeTe NW cross section obtained via aberration corrected STEM with evident trigonal crystal.

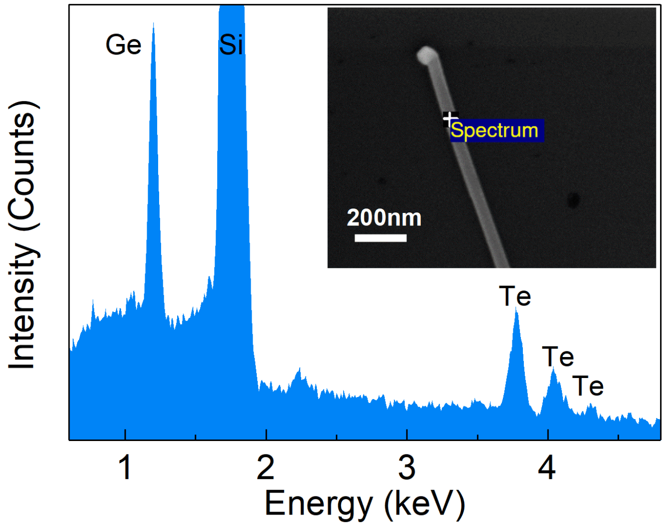


Figure S3. Energy dispersive X-ray spectrum of a GeTe nanowire and the corresponding SEM image.

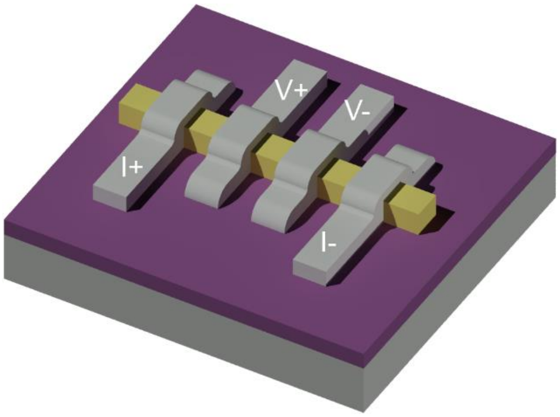


Figure S4. Schematic illustration of the 4-terminal measurement configuration

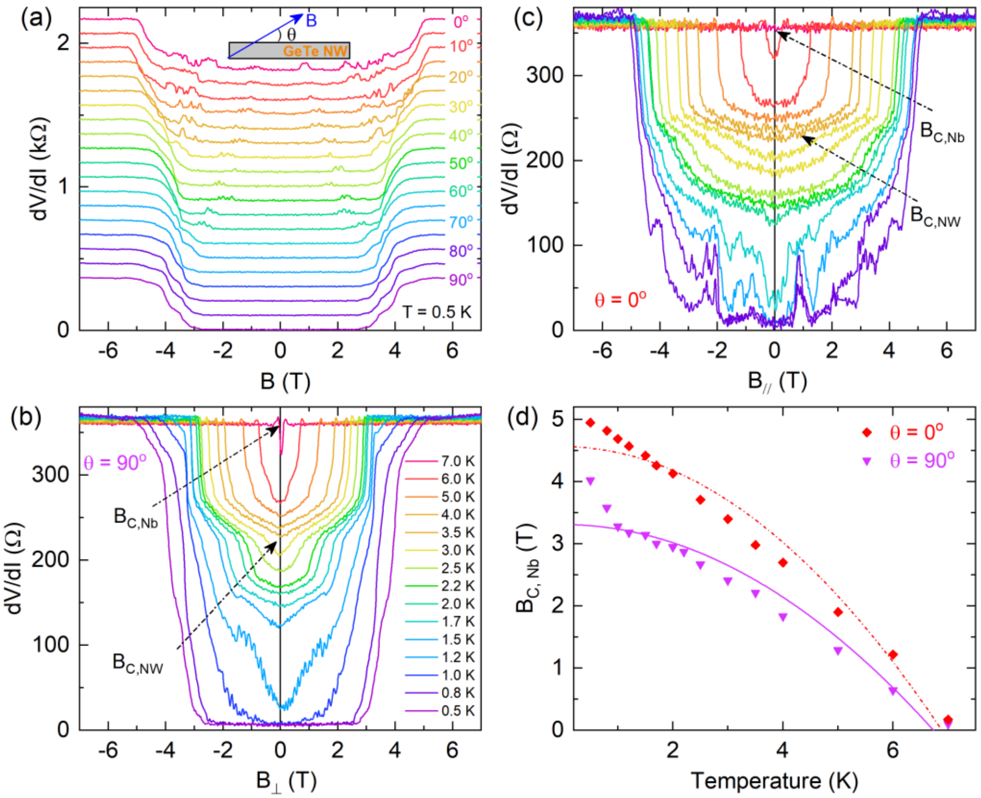


Fig. S5 (Color online) a) *dV/dI* of a Nb/GeTe/Nb junction for different tilt angles θ between magnetic field direction and nanowire axis at the temperature of 0.5 K. The inset depicts the definition of $\vartheta$ and the curves are shifted vertically for clarity. Temperature dependent *dV/dI* as a function of magnetic field at the angle $\vartheta$ of b) 90° and c) 0° at temperatures from 0.5 to 7.0 K. d) Temperature dependence of critical magnetic field $B_{C,Nb}$ of Nb contacts in the applied magnetic field at the angles θ of 0° and 90°.

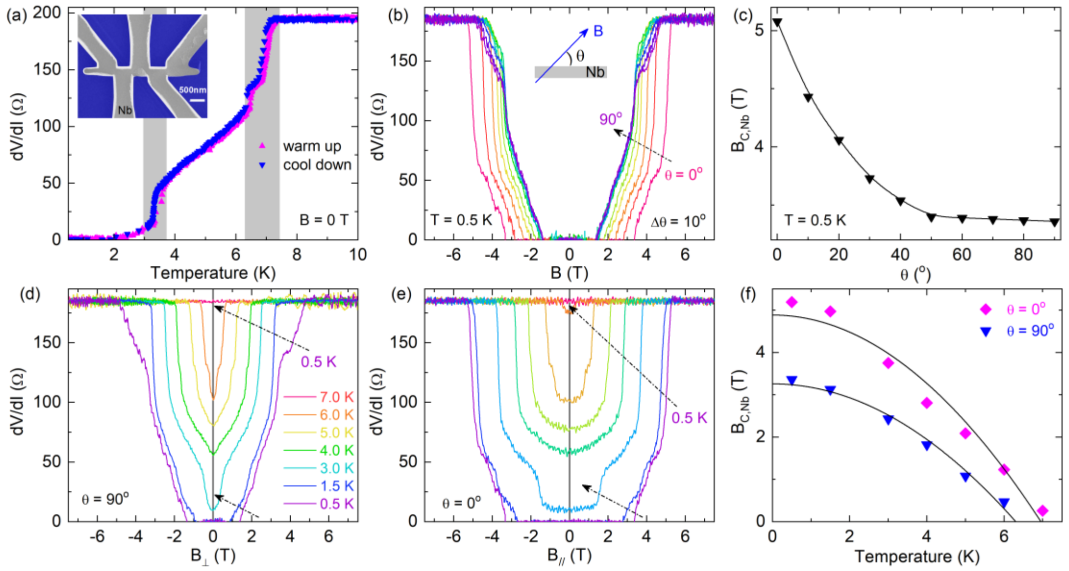


Figure S6. a) Four-terminal current-driven measurements of differential resistance dV/dI of a Nb/Nb-NW/Nb device (inset) during heating and cooling processes. b) Magnetoresistance dV/dI of the Nb/Nb-NW/Nb device, measured for different angles θ between magnetic eld direction and nanowire axis at 0.5 K. c) The critical magnetic field ($B_{c,Nb}$) of Nb lead as a function of tilt angle. The dV/dI as a function of magnetic field at the angles θ of d) 0 and e) 90 at temperatures from 0.5 to 7.0 K. f) Temperature dependency of experimental (dots) and tted (solid line) critical magnetic eld (Bc,Nb) at the angles of θ= 0° and 90°.
